# Supplementary material for: Probing octupolar hidden order via Janus impurities
Source: arXiv:2211.07666 source file (2024-02-15)
Supplement: Supplementary file 1 [file suppmat.pdf]

# SUPPLEMENTARY MATERIAL
# Probing octupolar hidden order via Janus impurities

Sreekar Voleti,[1] Koushik Pradhan,[2] Subhro Bhattacharjee,[3] Tanusri Saha-Dasgupta,[2] and Arun Paramekanti[1,2,3]

[1]*Department of Physics, University of Toronto, 60 St. George Street, Toronto, ON, M5S 1A7 Canada*
[2]*Department of Condensed Matter Physics and Materials Science, S.N. Bose National Centre for Basic Sciences, Kolkata 700098, India.*
[3]*International Centre for Theoretical Sciences, Bengaluru 560089, India*

(Dated: February 14, 2024)

### Supplementary Note 1: Phonon spectrum of $Ba_2Ca_{1-\delta}Na_\delta OsO_6$

The primitive unit cell of $Ba_2CaOsO_6$ contains a single formula unit, leading to a total of 30 phonon modes. Of these, there are 3 acoustic branches and 27 optical branches. Fig. 1(a) shows the low energy phonon spectrum of $Ba_2CaOsO_6$. For the sake of completeness, the irreducible representations (irreps) of the phonon modes at the Γ point are shown. It is to be noted that these are distinct from, and should not be confused with the notation used later discussing the local distortion modes of the $OsO_6$ octahedra. Aside from the three $T_{1u}$ acoustic modes, the full set of optical phonon modes (at higher energy, not shown) can be decomposed as follows: $\Gamma_{opt} = A_{1g} \bigoplus E_g \bigoplus T_{2u} \bigoplus 2T_{2g} \bigoplus 4T_{1u} \bigoplus T_{1g}$. Here, the $A$, $E$, and $T$ modes are singly, doubly, and triply degenerate. The four optical $T_{1u}$ modes are IR active, while the $A_{1g}$, $E_g$ and two $T_{2g}$ modes are found to be Raman active.

Fig. 1 (b) shows the low energy phonon dispersion of the $Ba_2Ca_{1-\delta}Na_\delta OsO_6$ structure with $\delta = 1/4$. Here, we have considered a cubic unit cell with 3 Ca and 1 Na (four formula unit cell) in the $Fm\bar{3}m$ structure. Upon introduction of Na in the structure, we find that the phonon dispersion develops an instability, signaled by negative phonon frequencies around the Γ point. This four formula unit cell hosts 120 phonon modes, out of which 3 are acoustic modes with $T_{1u}$ representation. According to the factor group analysis at the Γ point, the optical phonon modes belong to the irreducible representations: $\Gamma_{opt} = 4A_{1g} \bigoplus A_{2g} \bigoplus A_{2u} \bigoplus E_u \bigoplus 5E_g \bigoplus 8T_{2u} \bigoplus 6T_{2g} \bigoplus 14T_{1u} \bigoplus 5T_{1g}$. We find that the lowest $T_{1g}$ optic mode which was stable for $Ba_2CaOsO_6$ became unstable upon introduction of Na impurity. other modes being symmetry related. In order to understand the type of distortions which are stabilized in the Na substituted case, we next turn to the optimization of the crystal structure.

### Supplementary Note 2: Optimized structure of $Ba_2Ca_{1-\delta}Na_\delta OsO_6$

We first consider the unit cell, with one out of the four Ca atoms of $Ba_2CaOsO_6$ in cubic Fm-3m structure, replaced by Na (see Fig. 2a), amounting to $\delta = 1/4$, and optimize the structure fully. The optimization process creates two inequivalent Os sites. Os1 with site symmetry $4/mmm$ sitting at nearest neighbor position to Na, and another, Os2 with site symmetry $m-3m$ sitting far from Na in the cell. We note the Os2 site symmetry is same as that in pure Ca compound with four-fold rotation and a perpendicular mirror plane for the primary axis, three-fold roto-inversion symmetry for the secondary axis and two-fold rotation and a perpendicular mirror plane for the tertiary axis. For Os1 with lowered site symmetry, compared to Os2, while the primary direction has four fold rotational symmetry and a perpendicular mirror plane, the secondary and tertiary directions have two fold rotational symmetry and perpendicular mirror planes, generating local tetragonal distortion of the OsO6 octahedra. The distortion of $OsO_6$ octahedra can be measured by the distortion index, $D = \frac{1}{n}\sum_{i=1}^{n}\frac{|l_i - l_{av}|}{l_{av}}$ where $l_i$ is the Os-O bond-length of the $i$-th bond, and $l_{av}$ is the average bond length. The $D$ parameter of $Os1O_6$ is found to be about 0.01, while that of $Os2O_6$ is zero. To investigate the effect of impurity clustering, we expand the unit cell to a supercell of dimension $2 \times 2 \times 1$, resulting in 16 Ca sites in the cell. Two out of 16 Ca sites are replaced by Na, amounting to $\delta = 1/8$. Two configurations are considered, the near configuration and the far configuration. In the near configuration (cf Fig. 3), two Na atoms are placed at the nearest neighbor (NN) Ca positions of the $Ba_2Ca_{1-\delta}Na_\delta OsO_6$ structure. Optimization of this configuration leads to six inequivalent Os sites, Os1 . . . Os6. The Os atoms are found to have two or one or none Na atoms in the NN positions, no Na atom in the 2NN positions, and two or none Na toms in the 3NN positions. The distortion index of Os3 . . . Os6 are found to be one or two orders of magnitudes smaller, compared to that of Os1/Os2 . The site symmetry of Os1/Os2 is found to be $m2m/2mm$, which means two fold rotation and a perpendicular mirror plane for the primary/secondary and tertiary axis, while the secondary/primary axis has a two-fold rotation symmetry, mirror plane perpendicular to the corresponding axis being missing. Fig. 3(b)-(g) show the octahedral distortion at Os1-Os6 site, as well as their Na/Ca coordination. In the far configuration, (cf Fig. 4), two Na atoms are placed at the farthest Ca positions of the $Ba_2Ca_{1-\delta}Na_\delta OsO_6$ structure. Optimization of this

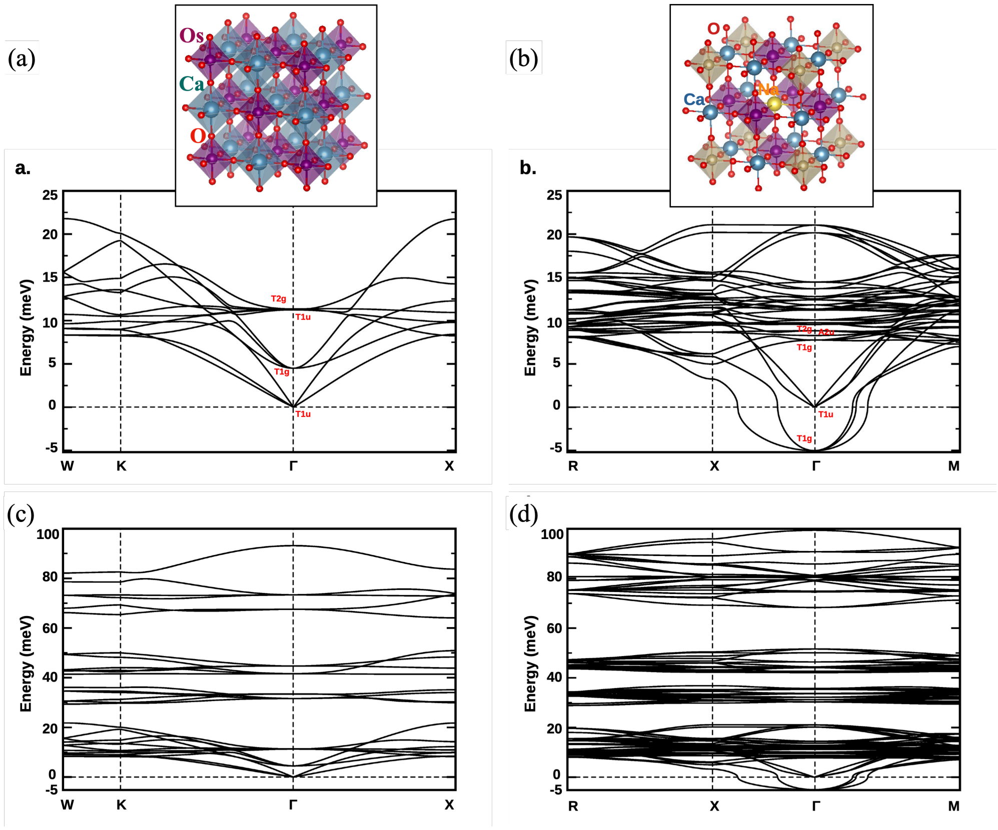


**Supplementary Figure 1:** **a.** Low energy phonon dispersion of $Ba_2CaOsO_6$ in the $Fm\bar{3}m$ structure, plotted along high symmetry path in the Brillouin zone of the primitive unit cell containing one formula unit. Inset shows the crystal structure, with cyan and purple octahedra representing $CaO_6$ and $OsO_6$ units. The irreps of the acoustic and optical phonon modes at the Γ point are indicated for a few low energy modes. All phonon frequencies are positive indicating the intrinsic stability of the structure. **b.** Low energy phonon dispersion of $Ba_2Ca_{1-\delta}Na_\delta OsO_6$ with $\delta = 1/4$ in the $Fm\bar{3}m$ structure, with inset showing the crystal structure. In this case, cyan and yellow balls represents the Ca and doped Na. There are two types of Os which have been marked using purple and grey octahedra. The dispersion is plotted along high symmetry path in the Brillouin zone of the cubic four formula unit cell. The irreps of the acoustic and optical phonon modes at the Γ point are indicated for a few low energy modes. In this case, we find negative frequency modes which underscore the instability of the $Fm\bar{3}m$ structure. **c.** Full phonon dispersion for $Ba_2CaOsO_6$ from panel **a**, with a total of 30 phonon modes, shown over the entire energy range. **d.** Full phonon dispersion for $Ba_2Ca_{1-\delta}Na_\delta OsO_6$ from panel **b**, with a total of total of 120 phonon modes shown over the entire energy range.

configuration leads to four inequivalent Os sites. The maximum distortion (0.01) in this case is found at Os1 class, with two Na atoms at its NN shell. The site symmetry of this maximum distorted Os site is found to be 4/mmm as discussed for $\delta = 1/8$.

### Supplementary Note 3: Multipoles in the $d^2$ configuration

For two electrons in the $t_{2g}$ orbitals, the ground state is a $J = 2$ moment, which we can view as arising from the the $j$-$j$ coupling between the two $j = 3/2$ electrons. This $J = 2$ moment is weakly split by additional symmetry allowed terms $H_{\rm CEF} = -V_{\rm eff}(\mathcal{O}_{40} + 5\mathcal{O}_{44})$. Here, the Steven's operators are given by

$$\begin{aligned} \mathcal{O}_{40} &= 35J_z^4 - (30J(J+1) - 25)J_z^2 + 3J^2(J+1)^2 \\ &- 6J(J+1), \quad (1) \\ \mathcal{O}_{44} &= \frac{1}{2}(J_+^4 + J_-^4). \quad (2) \end{aligned}$$

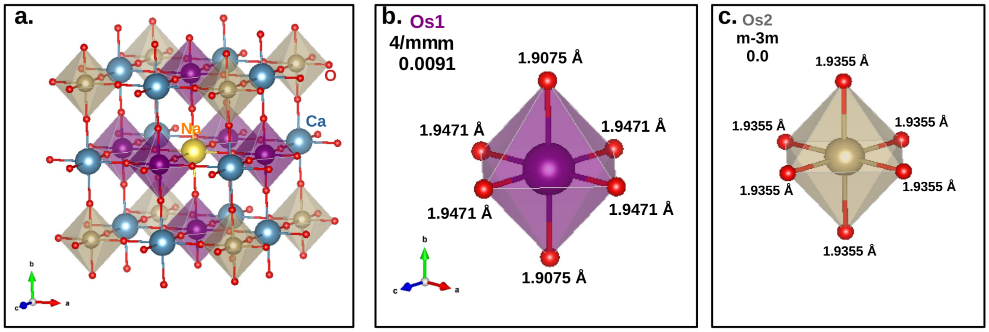


**Supplementary Figure 2:** (a) $Ba_2Ca_{1-\delta}Na_\delta OsO_6$ structure with $\delta = 1/4$, and impurity Na atom placed at the center of the cell. Deep cyan, yellow and red colored balls represent Ca, Na and O atoms, respectively. Two inequivalent Os sites are marked with differently shaded octahedra. (b) The bond length and bond angle variation of the distorted $Os1O_6$ alongwith Os1 site-symmetry and $D$ parameter, sitting close to Na. (c) The undistorted $Os2O_6$ octahedra, sitting far from Na atom.

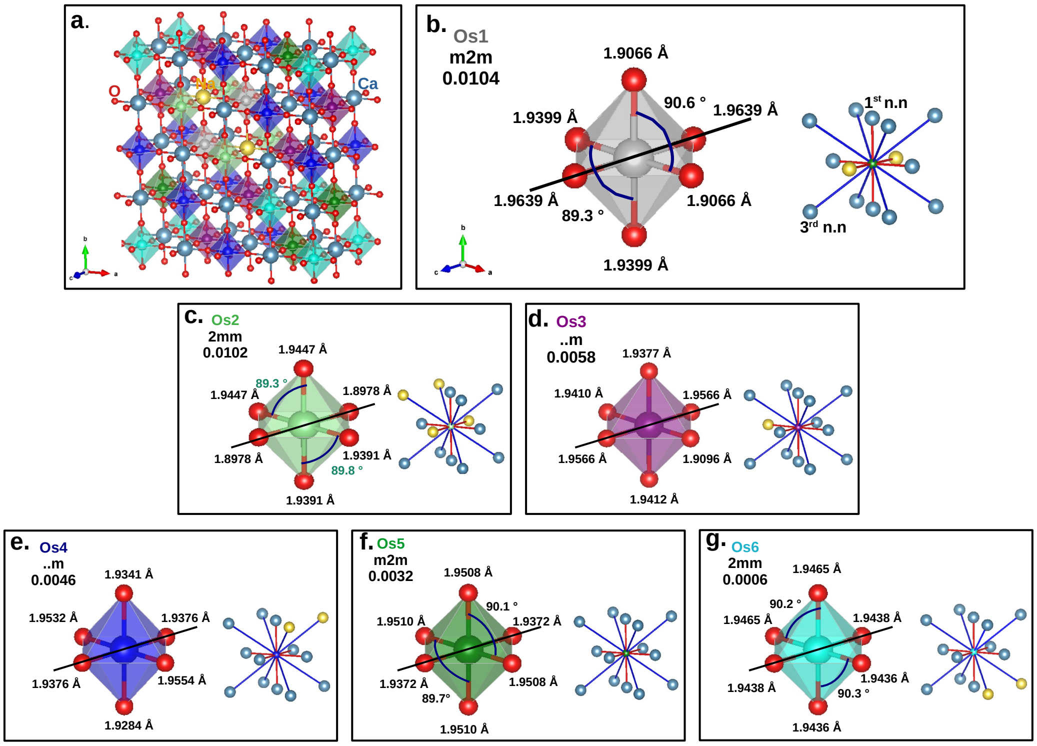


**Supplementary Figure 3:** (a) $Ba_2Ca_{1-\delta}Na_\delta OsO_6$ structure with $\delta = 1/8$, and two impurity Na atoms placed at NN B sites of the DP structure. Deep cyan, yellow and red colored balls represent Ca, Na and O atoms, respectively. Six inequivalent Os sites are marked with differently shaded octahedra. (b-g) The bond length and bond angle variation of the six different $OsO_6$ octahedra alongwith their site-symmetry and $D$ parameter. Shown are also the Na/Ca neighbor distributions surrounding the Os atoms at their 1NN and 3NN shell.

A nonzero $V_{\rm eff}$ only arises upon going beyond the simple $t_{2g}$ model and incorporating virtual excitations into the $e_g$ orbitals [1]. $V_{\rm eff} > 0$ leads to a non-Kramers ground state doublet, and an excited triplet with a small gap $\Delta = 120 V_{\rm eff}$. We have shown that $\Delta \sim \lambda^2 J_H / 10Dq$, where $\lambda$ is the SOC strength, $J_H$ is the Hund's coupling, and $10Dq$ is the $t_{2g}$-$e_g$ crystal field splitting [1]; a careful computation yields $\Delta \sim$ 10-20 meV, in reasonable agreement with the spin gap observed in inelastic neutron scattering experiments.

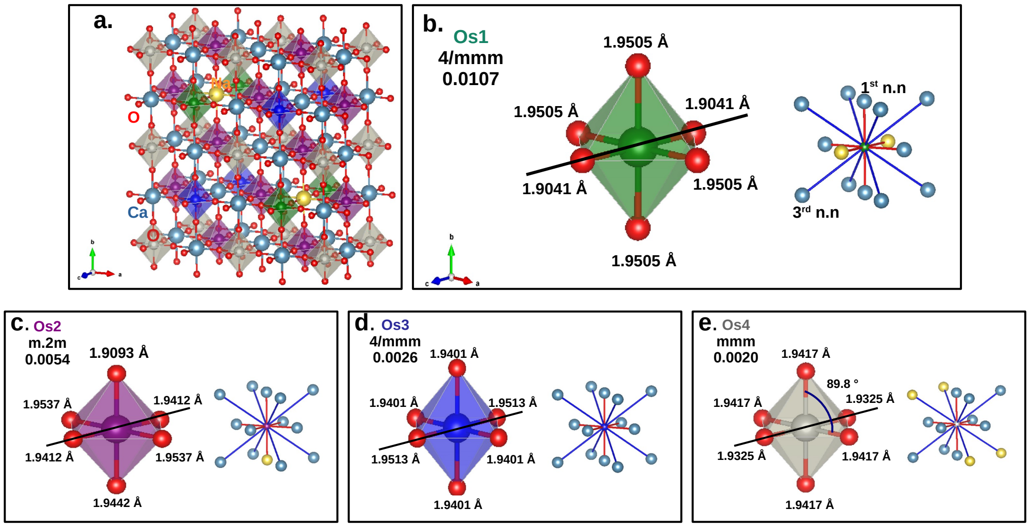


**Supplementary Figure 4:** (a) $Ba_2Ca_{1-\delta}Na_\delta OsO_6$ structure with $\delta = 1/8$, and two impurity Na atoms placed at farthest B sites of the DP structure. Deep cyan, yellow and red colored balls represent Ca, Na and O atoms, respectively. Four inequivalent Os sites are marked with differently shaded octahedra. (b-e) The bond length and bond angle variation of the four different $OsO_6$ octahedra alongwith their site-symmetry and $D$ parameter. Shown are also the Na/Ca neighbor distributions surrounding the Os atoms at their 1NN and 3NN shell.

Working in the $|J_z = m\rangle$ basis, the ground state non-Kramers doublet wavefunctions are given by

$$|\psi_{g,\uparrow}\rangle = \frac{1}{\sqrt{2}}(|2\rangle + |-2\rangle); \quad |\psi_{g,\downarrow}\rangle = |0\rangle, \tag{3}$$

while the excited triplet wavefunctions correspond to

$$|\psi_{e,\pm}\rangle = |\pm 1\rangle; \quad |\psi_{e,0}\rangle = \frac{1}{\sqrt{2}}(|2\rangle - |-2\rangle). \tag{4}$$

Within the non-Kramers doublet space, the Pauli matrices $\tau_x, \tau_y, \tau_z$ are proportional to multipole operators, given by $\tau_x \equiv (J_x^2 - J_y^2)/2\sqrt{3}$, $\tau_y \equiv \overline{J_x J_y J_z}/\sqrt{3}$, and $\tau_z \equiv (3J_z^2 - J(J+1))/6$. Here, $\tau_x, \tau_z$ are electric quadrupoles while $\tau_y$ is a magnetic octupole. The ground state doublet manifold has vanishing matrix elements for the dipole operators $\mathbf{J}$, precluding magnetic dipole ordering. However, the ground state doublet can lead to broken time-reversal symmetry below $T_c$ (while preserving cubic symmetry) if $\langle \tau_y \rangle \neq 0$ which corresponds to ferro-octupolar ordering.

## Supplementary Note 4: Computing multipolar exchange parameters

We compute the exchange parameters using the Schrieffer-Wolff transformation method outlined in Ref. [2]. From Density functional theory, we obtain the following local crystal field matrix (in eV):

$$A = \begin{pmatrix} -3.9496 & 0.0000 & 0.0000 & 0.0000 & 0.0000 \\ 0.0000 & -3.9496 & 0.0000 & 0.0000 & 0.0000 \\ 0.0000 & 0.0000 & -3.9496 & 0.0000 & 0.0000 \\ 0.0000 & 0.0000 & 0.0000 & 0.2429 & 0.0000 \\ 0.0000 & 0.0000 & 0.0000 & 0.0000 & 0.2429 \end{pmatrix} \tag{5}$$

To obtain the local spectrum, we supplement the above crystal field matrix with the following parameters:

1. Spin-orbit coupling $\lambda = 0.6$ eV
2. Hund's coupling $J_H = 0.5$ eV
3. Intra-orbital Hubbard interaction $U = 2.5$ eV

These parameters were chosen to obtain a local splitting of $\sim 15$ meV between the non-Kramers doublet ground state and the excited magnetic triplet. The intersite hopping matrix in the $xy$ plane, also obtained using DFT, is (in eV):

$$T^{xy} = \begin{pmatrix} 0.0395 & 0.0217 & 0.0000 & 0.0000 & 0.0000 \\ 0.0217 & 0.0395 & 0.0000 & 0.0000 & 0.0000 \\ 0.0000 & 0.0000 & 0.1174 & 0.0000 & -0.0661 \\ 0.0000 & 0.0000 & 0.0000 & 0.0000 & 0.0000 \\ 0.0000 & 0.0000 & -0.0661 & 0.0000 & 0.0000 \end{pmatrix} \tag{6}$$

## Supplementary Note 5: Determining the Local Strain Field caused by Substitution

### 1. *Field Magnitude*

The magnitude of the effective local strain field can be obtained from the single electron crystal field matrix. For an electron in a $d$ orbital, this will be a $5 \times 5$ matrix. A crude estimate of this matrix can be obtained using a point charge model of the $Os^{6+}$ ion with the octahedral cage of six oxygen atoms around it. The oxygen cage is represented by a potential $V(\mathbf{r})$, given by

$$V(\mathbf{r}) = \sum_{i=1}^{6} \frac{Z_{\mathrm{Ox}} e^2}{|\mathbf{r} - \mathbf{R}_i|}. \tag{7}$$

where $Z_{\mathrm{Ox}}$ is the charge on the Oxygen anions, and the Oxygens are numbered as in Fig. 1. As shown in Ref. [3], this expression can be written as a series expansion in spherical coordinates $(r, \theta, \phi)$ as,

$$V(\mathbf{r}) = \sum_{k=0}^{\infty} \sum_{m=-k}^{k} r^k \, q_{km} \, Y_{km}(\theta, \phi), \tag{8}$$

where $Y_{km}$ refers to a spherical harmonic, and

$$q_{km} = \left( \frac{4\pi Z_{\mathrm{Ox}} e^2}{2k+1} \right) \sum_{i=1}^{6} \frac{1}{a_i^{k+1}} Y^*_{km}(\theta_i, \phi_i). \tag{9}$$

In the above, $(a_i, \theta_i, \phi_i)$ refer to the spherical coordinates of the positions of each oxygen in the cage. Hence, distortions in the cage can be modelled by changing these coordinates in the expression. In what follows, we will keep terms in Eq. (8) up to order $k = 4$.

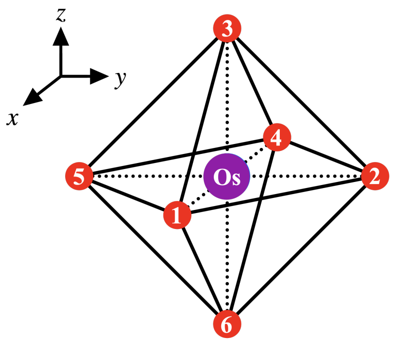


| Representation | Coordinate | Transformation properties | Expression |
|---|---|---|---|
| $A_{1g}$ | $Q_1$ | $x^2 + y^2 + z^2$ | $(y_2 - y_5 + z_2 - z_6 + x_1 - x_4)/\sqrt{6}$ |
| $E_g$ | $Q_{x^2-y^2}$ | $x^2 - y^2$ | $(x_1 - x_4 - y_2 + y_5)/2$ |
| $E_g$ | $Q_{z^2}$ | $3z^2 - r^2$ | $(2z_2 - 2z_6 - x_1 + x_4 - y_2 + y_5)/\sqrt{12}$ |
| $T_{2g}$ | $Q_{yz}$ | $yz$ | $(z_2 - z_5 + y_3 - y_6)/2$ |
| $T_{2g}$ | $Q_{zx}$ | $zx$ | $(x_3 - x_6 + z_1 - z_4)/2$ |
| $T_{2g}$ | $Q_{xy}$ | $xy$ | $(y_1 - y_4 + x_2 - x_5)/2$ |

**Supplementary Figure 5:** Left: Numbering of the oxygen atoms in the octahedral cage around the Os atom. Right: Table of relevant octahedral normal mode coordinates in terms of oxygen displacements. Reproduced from the full table in Ref. [4]

We will evaluate the expectation value of this potential in the manifold of $5d$ orbital wavefunctions $\psi_{nlm}$ with $n = 5$ and $l = 2$. These take the form

$$\psi_{n=5,l=2,m}(\mathbf{r}) = R_{n=5,l=2}(r) Y_{l=2,m}(\theta, \phi). \tag{10}$$

Here, $Y_{lm}$ is a spherical harmonic, and

$$R_{nl}(r) = \sqrt{\left(\frac{2Z}{na_0}\right)^3 \frac{(n-l-1)!}{2n(n+l)!}} \left(\frac{2Zr}{na_0}\right) \times \exp\left(-\frac{Zr}{na_0}\right) L_{2l+1}^{n-l-1}\left(\frac{2Zr}{na_0}\right), \tag{11}$$

where $Z$ is the nuclear charge, $a_0$ is the Bohr radius, and $L_\alpha^\beta$ is the generalized Laguerre polynomial associated with the hydrogen-like radial wavefunction.

Since $m$ ranges from $-2, ..., +2$, we will end up with a $5 \times 5$ matrix. Before employing this matrix in a single ion calculation, we transform into the orbital basis (see for example, the Appendix of Ref.[1]), where the complex spherical harmonics $Y_{lm}$ are replaced by real tesseral harmonics. We will refer to this matrix in what follows as the crystal field (CF) matrix. The basis for the CF matrix divides the states into the $t_{2g}$ and $e_g$ orbitals, as $\{yz, zx, xy, x^2-y^2, 3z^2-r^2\}$

Since we work with $5d$ orbital wavefunctions, the average $\langle r \rangle$ is in fact *bigger* than the Os-O spacings. While this means that the point charge model does not give extremely precise results, a rough estimate for the magnitude of the effect can still be determined. In what follows, we will take $Z = 7$, corresponding to an $Os^{6+}$ ion. In the undistorted case, we take all the Os-O spacings to be equal to $4a_0$ (corresponding to an equilibrium Os-O splitting of $a_{\text{Ox}} \sim 2\mathring{A}$), and have the angles $(\theta_i, \phi_i)$ given by $\{(\pi/2, 0), (\pi/2, \pi/2), (0, 0), (\pi/2, \pi), (\pi/2, 3\pi/2), (\pi, 0)\}$, listed in order of the the oxygen numberings given in Fig. . The CF matrix in this case takes the form (upto an overall constant):

$$A = V_{CF} \left(\begin{array}{ccc|cc} 0 & 0 & 0 & 0 & 0 \\ 0 & 0 & 0 & 0 & 0 \\ 0 & 0 & 0 & 0 & 0 \\ \hline 0 & 0 & 0 & 1 & 0 \\ 0 & 0 & 0 & 0 & 1 \end{array}\right) \tag{12}$$

where $V_{CF}$ corresponds to the splitting between the $t_{2g}$ and $e_g$ orbitals. We now consider a scenario where a Ca atom is replaced by an Na atom above the octahedron pictured in Fig. 1. This will cause a distortion along the $\hat{z}$ in such a way that Oxygen 3 has its Os-O spacing reduced to $(1-\varepsilon)a_{\text{Ox}}$. For small values of $\varepsilon$, the CF matrix takes the form

$$A = V_{CF} \left(\begin{array}{ccc|cc} -a\varepsilon & 0 & 0 & 0 & 0 \\ 0 & -a\varepsilon & 0 & 0 & 0 \\ 0 & 0 & -b\varepsilon & 0 & 0 \\ \hline 0 & 0 & 0 & 1-b\varepsilon & 0 \\ 0 & 0 & 0 & 0 & 1+c\varepsilon \end{array}\right), \tag{13}$$

where we find $(a, b, c) = (0.56\ ,\ 0.07\ ,\ 1.28)$. Note that a distortion along a different axis, and one which includes angle distortions, would lead to off-diagonal terms in the matrix in Eq. (13). We take this simple case for our ballpark estimate of the field magnitude scale. Using CF values from Ref. [2], we use $V_{CF} = 2.2$ eV. We can then use the methods outlined in [2] to obtain the single ion spectrum. Due to cubic symmetry being broken by the distortion, the non-Kramers doublet ground state will split, and we take half of this splitting as the magnitude of the effective strain field. In Fig. 6, we show the values of the non-Kramers doublet splitting for values of $\varepsilon$ up to 0.05.

We can see from Fig. 6 that we can expect the fields to have a scale of $5-10$ meV. In the main text, we consider a range of values, 5, 10, 20, and 30 meV. It should be noted that this large distortion field leads to the lowest excited triplet level coming close in energy to the higher non-Kramers doublet state. We continue to restrict ourselves to the doublet since the distortion manifests as a large pinning field, restricting us to the ground state.

### 2. *Field Direction(s)*

The strain can act as a field on the non Kramers doublet due to a linear vibronic coupling between moments of the doublet with normal modes of the octahedral cage. In order to determine the directions of the strain fields, we have

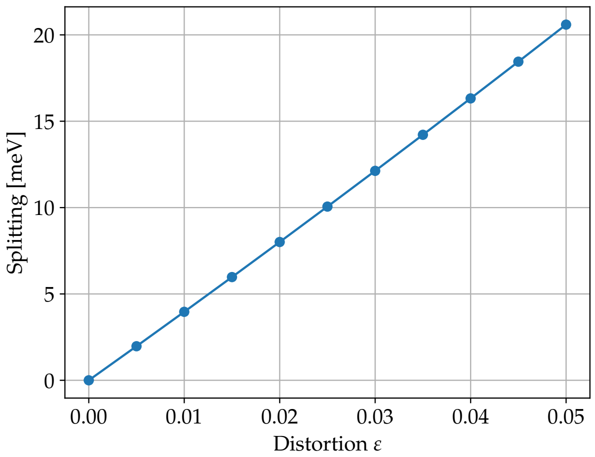


**Supplementary Figure 6:** Splitting between the non Kramers doublet states as a function of the distortion parameter $\varepsilon$. Note that the field magnitude is half that of this splitting.

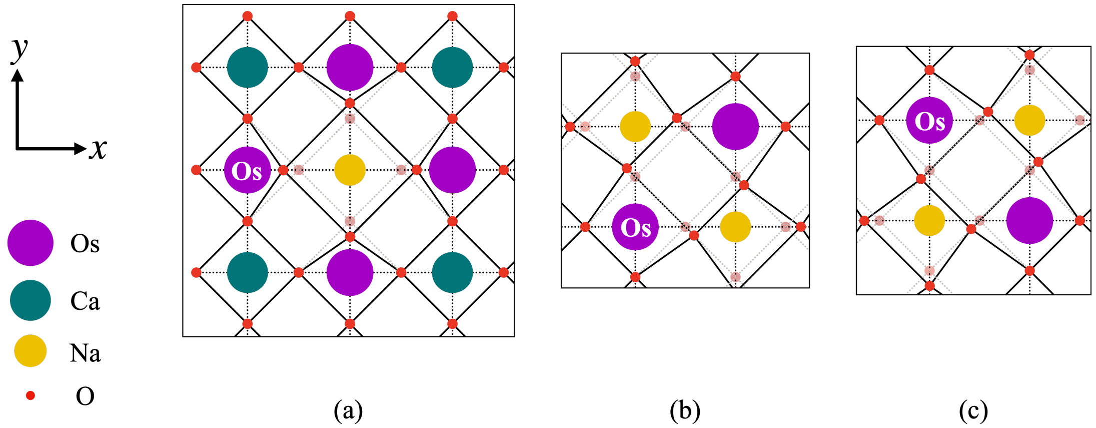


**Supplementary Figure 7:** (a) Single Impurity substitution. (b) Double impurity substitution Scenario A, (c) Scenario B. The lighter red circles depict the positions of the Oxygens in the ideal $Fm\bar{3}m$ (undoped) structure.

to represent the distortion in terms of the normal modes of the octahedral cage. These normal modes, by virtue of the cubic symmetry of the cage, can be classified into irreducible representations of the cubic group ($O_h$). Since the doublet has two $E_g$ quadrupole moments and an $A_{2u}$ octupole moment, if the decomposition of the distortion into normal modes contains displacements in these representations, they will act as fields on these moments. We define a set of six coordinate systems $((x_i, y_i, z_i)$ for $i \in \{1, ..., 6\}$, such that there is one centered on each Oxygen atom. In such a framework, the undistorted case corresponds to $x_i = y_i = z_i = 0$ for all $i$. We will look at the two types of substitution configurations discussed in the main text:

**Single Impurity Substitution:** We consider a single impurity, as shown in Fig. ??(a), which shows a zoomed in view of the distorted Os atoms around the isolated impurity in Fig. 3(b) of the main text. We consider the marked Os atom which experiences a distortion in the $\hat{x}$ direction (In the figure, this is the Os atom to the left of the Na impurity). Referring to Fig. 1, this corresponds to Oxygen 1 changing its Os-O distance, i.e. $x_1 \neq 0$. First, we write $x_1$ in terms of an inversion even and inversion odd term:

$$x_1 = \frac{1}{2}\left((x_1 - x_4) + (x_1 + x_4)\right). \tag{14}$$

Note that the first(second) term is inversion even(odd) since under inversion, $x_1 \to -x_4$ and $x_4 \to -x_1$. Since the non Kramers doublet transforms under an inversion even representation, once we project to the doublet, only the first term will survive. We can write this inversion even term in terms of the normal modes of the octahedral cage (see Table I and Ref. REF) and project to the inversion even representations to get:

$$x_1 \to \sqrt{\frac{2}{3}} Q_1 + Q_{x^2-y^2} - \frac{1}{\sqrt{3}} Q_{z^2} \tag{15}$$

where $Q_1$, $Q_{x^2-y^2}$ and $Q_{z^2}$ are defined in Table I. The first term, corresponding to an $A_{1g}$ normal mode, or a complete breathing of the octahedron, does not act to split the doublet, and hence does not take part in the effective field acting on the multipolar moments. The remaining terms act only on the $E_g$ quadrupole moments. The linear vibronic coupling allows for couplings only between distortions and moments that transform in the same way, the term in the Hamiltonian

$$V_{E_g} \left( Q_{x^2-y^2}\ \tau_x + \frac{1}{\sqrt{3}} Q_{z^2}\ \tau_z \right) \tag{16}$$

where $V_{E_g}$ is the strength of the vibronic coupling. In our simplified model, we assume $Q_{x^2-y^2} = Q_{z^2} \equiv Q$, such that the field term takes the form

$$\hat{x}\text{ Distortion } \to h \left( \frac{\sqrt{3}}{2} \tau_x - \frac{1}{2} \tau_z \right) \tag{17}$$

where $h = V_{E_g} Q/\sqrt{3}$. A similar analysis with $\hat{y}$ and $\hat{z}$ distortions gives

$$\hat{y}\text{ Distortion } \to h \left( -\frac{\sqrt{3}}{2} \tau_x - \frac{1}{2} \tau_z \right) \tag{18}$$

$$\hat{z}\text{ Distortion } \to h\tau_z \tag{19}$$

**Double Impurity Substitution:** In this section, we will show that double impurity configurations (as shown in FIG in the main text), are accompanied by a $T_{2g}$ distortion on the nearby Os atoms. This is due to the fact that neighboring impurty atoms lower the local symmetry, allowing for the Oxygen atoms around them to move in more directions. Below, we conduct the analysis in the $xy$ plane for concreteness. We must consider two scenarios, shown in Fig.7(b) and 7(c), corresponding to the case where the vector between the neighboring impurities $\mathbf{r}_{\text{Na}-\text{Na}}$ is $\pm(1, -1, 0)$ and $\pm(1, 1, 0)$.

**Scenario A ($\mathbf{r}_{\mathbf{Na-Na}} = \pm(\mathbf{1}, -\mathbf{1}, \mathbf{0})$) :** Consider the marked Os atom in Fig. 7(b). Based on the Oxygen numbering in Fig. 4, we can read off from the diagram that $x_1 > 0$, $y_1 < 0$, $x_2 < 0$, and $y_2 > 0$. Referring to Table 1, the $x_1$ and $y_2$ displacements can be written in terms of normal modes discussed in the preceding section ($Q_1$, $Q_{x^2-y^2}$, $Q_{z^2}$), but the introduction of nonzero $x_2$ and $y_1$ displacement means that the $Q_{xy}$ normal mode, which transforms under the $T_{2g}$ representation of $O_h$ comes into play. Since $x_2 < 0$ and $y_1 < 0$, we conclude that $Q_{xy} < 0$. This implies that in such an impurity configuration, the local strain tensor will have a component $\varepsilon_{xy} < 0$. It can be checked that the same is true for the other Os atom in the figure.

**Scenario B ($\mathbf{r}_{\mathbf{Na-Na}} = \pm(\mathbf{1}, \mathbf{1}, \mathbf{0})$) :** We repeat that analysis above, and see that for the marked Os atom in Fig. 7(c) has oxygen displacements $x_1 > 0$, $y_1 > 0$, $x_5 < 0$, and $y_5 < 0$. Again, the nonzero $y_1$ and $x_5$ give rise to a $Q_{xy}$ distortion, but this time such that $Q_{xy} > 0$, and by extension, $\varepsilon_{xy} > 0$.

We have thus shown that when we have neighboring impurity atoms, there is a $T_{2g}$ strain applied on the nearby Os atoms, with the sign of the strain being dependent on the specific arrangement of the impurities.

### Supplementary Note 6: Raw histograms used to generate simulated NMR spectra

Below, we present the raw histograms from which the simulated spectra weer produced. As mentioned in the main text, we average over 20 impurity configurations, and over 300 separate Zeeman field orientations. Since this was done on at $\delta = 0.1$ on a $14 \times 14 \times 14$ cluster, the number of data points is $0.1 \times 14^3 \times 100 \times 300 \times 3 \approx 8 \times 10^6$, where the last factor of 3 comes from the fact that each Na atom's local Hamiltonian gives three frequencies.

### Supplementary Note 7: Coupling of magnetic field to the non-Kramers doublet

For completeness, we also derive the coupling of the external magnetic field $\mathbf{B}$ to the low energy doublet, we start from a microscopic Hamiltonian $H_B^{\text{mic}} = g\mu_B \mathbf{B} \cdot \mathbf{J}$ with the Landé g-factor $g = 1/2$. We note that the dipole operator

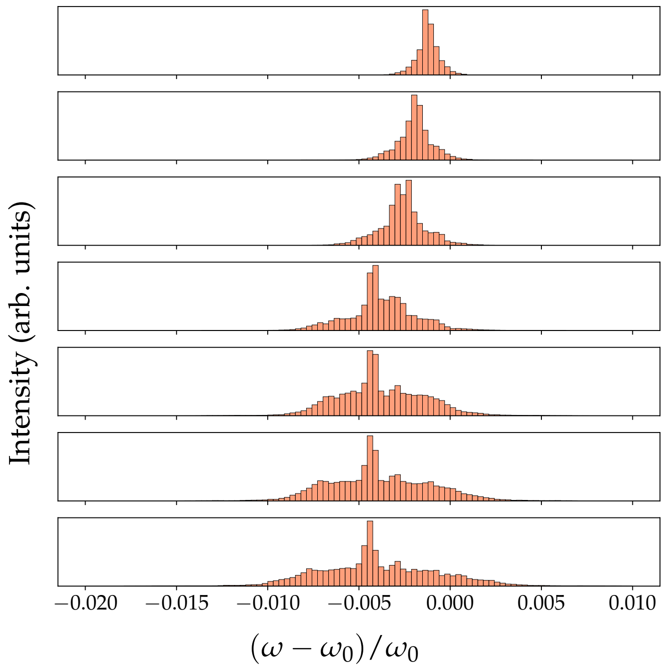


**Supplementary Figure 8:** Raw histograms

has no matrix elements within the low energy non-Kramers doublet space, but it couples the ground doublet to the excited triplet. To obtain its leading order effect on the low energy doublet, we thus carry out a second order perturbation theory calculation, and find

$$H_B^{\rm eff} = -\alpha\left[\sqrt{3}(B_x^2 - B_y^2)\tau_x + (3B_z^2 - B^2)\tau_z\right] \quad (20)$$

$$\equiv -h_x\tau_x - h_z\tau_z \quad (21)$$

where the coupling constant $\alpha = (g\mu_B)^2/4\Delta$. The magnetic field couples directly to the octupolar component only at $\mathcal{O}(B^3)$, so we omit this coupling. Fixing $\mathbf{B} = B\hat{n}$, we arrive at

$$h_x = \alpha B^2\sqrt{3}(n_x^2 - n_y^2) \quad (22)$$

$$h_z = \alpha B^2(3n_z^2 - 1) \quad (23)$$

Plugging in $\mu_B \approx 0.058$meV/T and $\Delta \approx 20$ meV, we find $\alpha \approx 10^{-4}$meV/T$^2$. Setting $B = 10T$, the energy scale of the 'transverse field' is $\alpha B^2 \approx 0.01$ meV. The impact of the applied magnetic field $B$ is thus much weaker than the typical exchange scales, $T_c$, and impurity induced transverse quadrupolar fields, and thus cannot itself significantly impact the multipolar orders.

[1] S. Voleti, D. D. Maharaj, B. D. Gaulin, G. Luke, and A. Paramekanti, Multipolar magnetism in $d$-orbital systems: Crystal field levels, octupolar order, and orbital loop currents, Phys. Rev. B **101**, 155118 (2020).
[2] S. Voleti, A. Haldar, and A. Paramekanti, Octupolar order and Ising quantum criticality tuned by strain and dimensionality: Application to $d$-orbital Mott insulators, Phys. Rev. B **104**, 174431 (2021).
[3] S. Sugano, Y. Tanabe, and H. Kamimura, *Multiplets of Transition Metal Ions in Crystals* (Academic Press, New York and London, 1970).
[4] I. B. Bersuker and V. Z. Polinger, *Vibronic Interactions in Molecules and Crystals* (Springer, Berlin, Heidelberg, 1989).
